# Supplementary material for: Towards an efficient and risk aware strategy for guiding farmers in identifying best crop management
Source: arXiv:2210.04537 source file (2022-10-10)
Supplement: Supplementary file 1 [file ideas.tex]

\subsection{Algorithm}

A proposition of experimental process that could be interesting to test. We could either directly start with the simulator or with toy data (should be better to test several config)
\begin{enumerate}
\item Collect the set of (discretized) prior distributions $F_1, \dots, F_k$ as a two vectors $(x_{1}^k, \dots, x_N^k)$ and a set of frequencies $f_k = (f_1^k, \dots, f_N^k)$. The discretization can be made with fixed bin size or fixed frequency.
\item First step: We run CVTS with the prior distribution. The mean of the Dirichlet distribution is $\rho f_k$. Simple version: $\rho$ is set manually. Other possibility: $\rho$ calibrated such that the outcomes fit a risk-budget defined by the users.
\item B-CVTS step: Once the mean vector is defined we run the algorithm as usual. We obtain the $M$ actions.
\item Assign the actions according to some rule (at random, equalizing the risk taken, etc)
\item Observe rewards
\item Update the weight of the prior: likelihood ratio, or any sequential update procedure (or simply decreasing weights). 
\end{enumerate}

\section{Notes Literature Dorian}

\subsection{Improving offline evaluation of contextual bandit algorithms
via bootstrapping techniques (Nicol, Mary, Preux)}

\paragraph{Setting:} Contextual bandits, before implementing the algorithm irl we want to test it on an available dataset $\cS$ of size $\cS = T$ of triplets $(x_t, a_t, r_t)$ (context/action/reward), assuming that actions have been chosen uniformly at each time. 

\paragraph{Contribution:} The baseline is called \textit{Replay} and consists in screening the dataset, observing the context $x_t$, choosing an action and observing the reward \textit{only if it is the actual action used in the dataset}. This way, actually $\approx T/K$ data are used. To overcome this, the authors implement Replay on $B$ \textit{bootstrapped} datasets of size $KT$, with some additional noise in contexts called jittering. They prove nice statistical properties and show the benefits of this approach in experiments, w.r.t vanilla Replay.

\paragraph{My Comment:} Not sure if it is relevant for us: the main issue is the finite size of the dataset, which is not our case as we agree that we could virtually perform as many experiments as we want in sillico. Furthermore, I am not sure to really understand the interest of using the dataset by running a bandit algorithm on it: is it to compare the regret of different bandit algorithms and then choose the one that compares favorably in the offline setting? Because if this is just to "boost" the algorithm that will be used in the real system I do not understand why we don't just take all the data and simply initialize the bandit algoritm irl with estimators computed on all these data. 
Again, with potentially infinite number of simulation the "comparison" between bandit algorithms can be performed in our case the way we did in the paper's experiments (and we can consider the question is answered with CVTS being clearly better). And on the other case I am not sure it is the most clever way to introduce prior knowledge in our system, for our specific application.

\subsection{Safe Policy Improvement by Minimizing Robust
Baseline Regret}
https://proceedings.neurips.cc/paper/2016/file/9a3d458322d70046f63dfd8b0153ece4-Paper.pdf

\paragraph{Objective:} Historical data allows to build an estimate of the transition probabilities in a MDP problem. We want to implement a policy that improves the model build with historical data (= increase the value of the policy). Cool idea: consider the perf of baseline/improved policy at each state to change the policy state by state.

\paragraph{Comment:} Interesting but not sure how it can be applied to our problem. It seems that the paper consider estimation of the transition probabilities, while we could get a complete estimation of the rewards distributions. As the previous article, I think our simulator would make much more information available than what the article considers in its hypothesis.

\subsection{Compliance-aware bandits}

https://arxiv.org/pdf/1602.02852.pdf

\paragraph{Objective:} People often do what they're told. Sometimes this can carry some information, that can be used by the bandit algorithms. Authors claim that it is better to use this info than to naively run the bandit algorithm.

\paragraph{Comments:} The main point is that the underlying population may be divided into sub-populations with different behaviours/bias. 3 approaches are proposed for the reward evaluation: 1) Chosen, where the bandit gives the observed reward to the arm it chose, whatever the compliance state, 2) Actual, the bandit gives the reward to the true arm from which it has been collected, 3) Comply, only take the reward if compliance was respected.
Hierarchical Bandit: A bandit algorithm chooses to play protocol (1), (2) or (3). Another bandit algorithm is associated to each protocol, and updated following the chosen protocol. Exp3 is used as the top bandit (not stochastic).

Intéressant en vrai.

\RG{Another remark on compliance: a farmer is unlikely to strictly follow, say for a given planting date, all crop management. For instance, depending on soil fertility a local adjustment might be required. Some might need to fertilize more than other. For our purpose we can average it, but we should be careful with unbalanced treatments in samples... It is unclear for me if an high fertilization vs a low fertilization treatment could be considered as a part of a context, or as an action combination e.g. sowing date 1 x low fert, and then with an anova like the effect of the fertilization removed to only keep the effect of sowing date}

\subsection{Stochastic Bandit with context distributions}

https://proceedings.neurips.cc/paper/2019/file/a6b964c0bb675116a15ef1325b01ff45-Paper.pdf

\paragraph{Objective:} Contextual bandits, but sometimes the learner cannot have access to the precise context before the action choice. The motivational example is of great interest for us, consider that we have weather forecasts: we can associate it to a distribution of contexts (i.e the actual observed weather at the time of realization). Then, each context can be associated with an expected reward according to some model. Authors provide an algorithm and theoretical guarantees in the special linear case.

\paragraph{Comments:} Very cool and pleasant to read paper, everything is quite intuitive. My main remarks are about the application to our setting: 1) if we get weather forecast we have to associate them to a distribution of weather: will we have enough data to do that? If we have to take a decision in advance for planting date, it is sure that the uncertainty of weather forecasts will not be the same for each date (increasing uncertainty), how do we implement that? 2) the authors warn that guarantees are not achievable for any context distributions/associated mean rewards, with a very simple non learn-able example. This means that we will need to put a precise model on the contexts/means, considering that being non-parametric is at the core of our work how can we manage that? Furthermore, what is the regularity of the reward distributions with respect to the contexts?

\subsection{Compte-rendu de la réunion}

Some keywords for our research: group testing, Batch learning (even with adaptive group size), Offline evaluation, Structured bandits, matching of time series, contextual bandits, learning with dependent arms, sequential regression...

We have to precisely refine what we want to do, because they are many possibilities.

\section{Notes sur la doc DSSAT de Romain}
Différents settings :
\begin{enumerate}
    \item Simple bandits
    \item Contextual Bandits
    \item Case-based: comparing with past year information + 3 month weather data (=context)
    \item More complex pb: we choose the full crop-management plan, and have a double objective.
\end{enumerate}

In the paragraph below I denote (x) the item in the previous list and x. those from the list of essential features. 

\paragraph{Setting (1)} Simple bandits is handled by CVTS, and we could easily integrate 1. and 4., and we already discussed about 3. and can continue to try different solutions. 

\paragraph{Setting (2)} I don't see how (2) is a contextual bandit in the strict sense, as the contextual information does not change for a given field (or should it?), thus it seems pretty similar as (1) to me. I guess the idea was to perform simultaneous recommendations to different fields? If this is the case we have to find a model to use knowledge from different (let say $M$) fields. Without such assumption we can only train $M$ not-interacting bandits. Simple solution = clustering and training $M'<< M $ bandits. More sophisticated = see literature (e.g assume $\mu_k(x_m)$ for each date $k$ context $m$ and some particular structure in $\mu_k$).

RG: contextual in the sense that a different farmer ask a recommendation at each time. We receive her soil information before running the algorithm. We can have significant differences in the same region (depth, sandy soil,...). Can make the signal noisy if not taken into account. 

\paragraph{Setting (3)} by past year observations you mean all climate data and yields, or more? And for the current data you mean only \textit{observed} data and not \textit{predictions}? This time it looks indeed more like a real contextual bandits. Usually we assume a model on the means according to the context. For what I know, it is often parametric but I am not a specialist of this literature. I will check if contextual bandits are a thing for non-parametric distributions (should be the case at least for bounded).
 
\paragraph{Setting (4)} if we consider a full management plan, I guess there should be some sort of structure between the outcomes of each plan. See which one should be relevant, however some processing may be needed because I guess not all actions should have the same impact on the outcome. I also the case of the double objective can be handled quite trivially by mapping the observed data into a scalar objective (let say $r_1-\lambda r_2$), or something like that. I don't think it would change many things if we choose to learn the distribution of the mapping, however if try to learn the two distributions we have to take into account the correlation structure.

\paragraph{Bilan} So in my opinion, setting (1) is simple but is the setting that can allow us to directly consider problems 1. -> 4. Setting (2) is pretty closed and could be simply provided in the batch setting (if I understand correctly). Settings (3) and (4) are also cool but are different bandit problems and I don't think CVTS will be what we need (or maybe on top of something else, but we will need to discuss together more precise hypothesis).

\paragraph{Réunion Romain:} Batch size is not a degree of freedom we have, while literature focus on controlling the batch size (finding the optimal + several steps). Not in control of the batch size, given data + not in control of compliance. The can question that can be raised is the one of the diversity of actions among farmers (should bring positive aspects). The main problem raised by batches is that results will be correlated (example: high correlation at the scale of a département). Context = a fixed effect (e.g: soil + past already observed meteorological data) + a random effect of the future meteo: we can use the setting of Kirschner to handle prediction, we have to know a true climate distribution associated with predictions.

The main question is: how do we implement the context ? We have to better understand how soil condition affect the mean and if we can catch an easy structure. If not, we can think of clustering the contexts, or using methods as Kernels and GP (see Audrey Durand works).

\subsection{Notes avant réunion lundi}

Observations sur les distribs envoyées par Romain:

\begin{itemize}
    \item Il y a généralement 3 modes: (1) une proba de récolter 0, (2) un mode "bas", et (3) un mode "haut", les 3 étant plus ou moins piqués. L'écart entre 0 et le mode "bas" a l'air à peu près constant, peut-être est-ce une feature apprenable. Pour le mode haut ça semble variable en revanche.
    \item Peut-être qu'un modèle de mixture pourrait marcher: nombre finis de paramètres, chacun avec une dépendance dans le contexte. Example: $Y= (1-\bP(Y=0|X))(p_1 \nu_1 + p_2 \nu_2)$, avec $\bP(Y=0|X)= f(\theta^t X)$, $\nu_1$ qui serait peut-être un truc genre gaussien, et $\nu_2$... je sais pas. Sinon avec une hypothèse bornée on pourrait aller sur des lois beta, avec ça il y a peut-être moyen de fitter les distribs bizarre, mais bon ça fait genre 7 paramètre à apprendre...
    \item Il semble y avoir une structure de type unimodalité (à peu près quelque soit l'objectif semble-t-il). Cela serait-il toujours le cas?
    \item Dans les exemples envoyés la dernière date est toujours la meilleure, ça serait bien de voir des cas où ça ne serait pas le cas (pour checker cette hypothèse d'unimodalité)
\end{itemize}
    
Quelques papiers qui peuvent être intéressants sur non contextual bandits:
\begin{itemize}
    \item "https://papers.nips.cc/paper/2019/file/aceacd5df18526f1d96ee1b9714e95eb-Paper.pdf", assumption = reward response to context is Lipschitz, context sampled uniformly in the unit ball and gaussian rewards (mean + gaussian noise).
    \item "https://arxiv.org/pdf/1801.01750.pdf": idem, lipchitz + subgaussian noise. KNN + UCB
    \item "http://proceedings.mlr.press/v124/bibaut20a/bibaut20a.pdf" reward bernoulli. MAIS: ils se posent la question de la complexité d'un espace de contextes, qui peut nous inspirer.
    \item "https://www0.gsb.columbia.edu/faculty/azeevi/PAPERS/banditCOLT4.pdf" toujours le même type de contextual structure.
\end{itemize}

Réflexions après ces lectures: important de définir dans quoi évoluent les contexte -> sont-ils discrets ou continus? Quelles valeurs prises? Les contextes continus sont-ils discrétizable ou ça vaut la peine de les considérer de manière continue (sachant qu'il va y avoir une uncertainty j'imagine).

Ce qui est compliqué c'est que les approches que je découvre considèrent tous reward = fonction du contexte + white noise. Dans notre cas c'est très clairement impossible! Par exemple, on pourrait ne pas changer la moyenne (donc déjà merci pour trouver une fonction qui va) mais changer la proba en 0 et la upper tail!

Article potentiellement intéressant: TS with sparse GP, "https://arxiv.org/pdf/2006.05356.pdf"

Trucs cools: 

\begin{itemize}
    \item Risk-aversion: risk-constrained ou CVaR
    \item "prior": offline data + simul
    \item Contexte: grande dimension, comment synthétiser les contextes? Modéliser leurs effets? Representation learning.
\end{itemize}

Problème qu'on veut résoudre;

\begin{itemize}
    \item User: veut une reco perso qui prend en compte son aversion au risque = plan de fertilisation du blé 
    \item On veut utiliser : toute la donnnée contextuelle connectée = user info + agronomique
    \item On veut améliorer cette reco au fur et à mesure des infos
    \item Objectif: limiter ces erreurs avec les modèles agro et les infos déjà dans les bases de données
    \item à chaque saison: $n$ agri vont demander des actions, on veut aller voir ce qu'ils ont fait et ce que ça a donné. 
    \item Récompense = expert-provided, rendement grain + budget pollution (ou pénalité).
    \item -> Bandits risk-averse, données offline + simulateurs disponibles, collection de rewards bandit-like.
\end{itemize}

On veut savoir si nos solutions sont applicables dans la vraie vie. 

Lui: Gym-DSSAT c'est quasiment good, après il se met full time dessus.

\newpage 

\subsection{Ideas for the new direction}

We first define the problem we try to answer more precisely. First, the objective is to provide recommendations to farmer, where each recommendation can be represented by an arm in a multi-armed bandit problem. Once a decision is taken, several months are needed to observe the result. Fortunately, we will be able to recommend to several farmers simultaneously, which will give access to a relatively large amount of data. We decompose the problem into several layers of complexity, that we plan to address one after the other:

\begin{enumerate}
    \item \textbf{Risk-aware} decisions for a \textbf{batch} of different farmers. Without more assumptions we can choose the CVaR or Risk-constrained bandit framework and apply B-CVTS. The fact that B-CVTS is a random algorithm is good for batch recommendation, as for instance a UCB would recommend the same action to each farmer. Still on this simple problem, we could ask ourselves if the problem could not be \textbf{unimodal}, i.e arms have a graph structure and there exists a path of increasing quality arms up to the best arm (we can then investigate solutions locally). The adaptation of CVTS to unimodality would be naturally to run CVTS on a neighborhood of the current best empirical arm.
    \item \textbf{Use contextual information}: We can get quite "high" dimensional data, can be user information (soil conditions, use of engrais and pesticide, previous years' data) or expert information. First, we could question if the data can be synthesized into low dimensional vector, which would certainly be better for the learning algorithm. Furthermore because many variables can be correlated. Check if a simple \textbf{PCA} or \textbf{matrix factorization} algorithm can be used. Then, we have to decide the \textbf{influence of the context on the rewards' distributions}. As we are facing non parametric distribution with heteroscedastic noise, we can first opt for an \textbf{online clustering} algorithm, running independent bandit algorithms on each cluster. After that, we could try more sophisticated solutions (\textbf{Gaussian Process}?)
    \item \textbf{Use offline data and simulators for "Safe" RL}: each efficient bandit algorithm suffers from a certain amount of "uniform exploration" at the beginning. We would really like to avoid this in practice, hence we want to pre-train our algorithm in sillico. However, their may be a gap between the "true" distributions and the distributions captured by the data/simulator. Hence, how can we transfer some knowledge learned offline while letting enough room for adaptation in case of mismatch? This topic seems quite new.
\end{enumerate}

We would like to focus on these three inter-dependent problems. We claim that (1) is mostly solved on a practical point of view, (2) and (3) appear more complex and could be treated in any order, but it seems logical to including the clustering part in (3) hence the order of the presentation.

\subsection{Contextual information in non-parametric risk-aware learning}

\subsubsection{Literature: Gentile paper}

http://proceedings.mlr.press/v32/gentile14.pdf .

\paragraph{Setting} Online clustering in linear bandits. Idea: at each time a general context $i_t \in V$ is drawn, with $V = \cup_{j=1}^m V_j$ and $|V| = n \gg m$. We associate $i_t$ with the set of arms $C_{i_t} = (x_{t, 1}, \dots, x_{t, c_t})$, the learner chooses an arm $y_t$ and observes $a_t = u_{i_t}^T y_t + \epsilon_t $. If 2 arms are from the same cluster they share their parameter $u_i$.

\paragraph{Algorithm} The proposed algorithm uses classic parameter estimation, and combines it with a simple confidence-based clustering scheme. At the beginning all contexts are given in a fully connected graph, and we sequentially remove some edges. In short, we have different blocks:
\begin{enumerate}
    \item Given a clustering, compute estimators (classic OLS) of a cluster's parameter by aggregating all data from this cluster's arm. Decide which arm to sample accordingly.
    \item Maintain individual estimators of the parameter of \textbf{each} context parameter. If the distance between two parameters is larger than a certain confidence delete the edge between the two contexts. 
\end{enumerate}

Note that this way we consider a finite set of contexts, and they are only defined by their unknown parameter.

\paragraph{Comment} The linear bandit setting is convenient for clustering, because we know "what to look at" to characterize the reward distribution of each context, thanks to the parameter vector. Our setting is a bit different: we have a precise characterization of this parameter (or at least we could map the context data we get into such parameter), but again not a clear link between this parameter and the reward distribution. Furthermore, the idea of succesfully removing edge is cool, but there does not seem to be a way to recover lost edges. If we have continuous contexts we may want to focus on algorithms providing clear frontiers between clusters.

\paragraph{Thoughts after reading this article} Continue to maintain independent estimators for the reward distributions given each individual contexts seems a good idea. The contrary of what they do may be appropriate: start with a (potentially large) number of expert-chosen clusters, and then sequentially merge different clusters. Also, define the clustering through a metric that is \textbf{chosen according to the reward}: what they do is essentially saying that contexts from the same structure share the same mean. We could provide a first algorithm that would do the same for (1) the mean, (2) CVaR, (3) the probability of poor (zero) harvest, (4) the parameters of a mixture model, (5) some chosen quantiles/order statistics... Of course each of them should require different kind of tests. We may use confidence regions for most of them (except maybe (4)).

Imagine we choose statistics such that it is possible to compute confidence balls. Assume that we start with some clusters $C_1, \dots, C_M$ given by a previous iteration, satisfying $\R^d = \cup C_i$. At the end of the data collection phase we want to check two factors: (1) do we want to split some cluster in 2/more clusters? (2) do we want to merge clusters ? (consider the smaller cluster resulting from step (1)).

\RG{how do we treat uncertainty in contexts? Context information is subject to uncertainty as well! Does it only add to reward noise?}
\DB{Good question! It depends of the granularity we decide to choose in the clustering, if we decide to already put each context into a (potentially large number) of un-splittable balls then this is only a problem at the frontier. If we decide to use the full "continuousness" of the contexts well... it depends if we are able to "quantify" this uncertainty. Would you be able to draw a confidence ball around this context? If so, what do we do: re-sample uniformly in this ball? choose the more "exploratory" context in this ball? \\
Otherwise, could we have a generative model? \\
In my opinion we could start by acting as if contexts were deterministic.}
\RG{I agree. We have to state that context are, in practice, subject to uncertainty. Nevertheless, it would be complicated to measure that uncertainty. Example: for soil measurements that would be possible. But for human observations? Would be too costly. As well, some data may be inferred. It would require a very complicated process.}
