# Supplementary material for: Towards an efficient and risk aware strategy for guiding farmers in identifying best crop management
Source: arXiv:2210.04537 source file (2022-10-10)
Supplement: Supplementary file 2 [file weather.tex]

In this section, we detail the parameters, based on historical weather records, used by WGEN (\cite{richardson1984wgen} and \cite{soltani2003statistical}) to generate stochastic weather. For each of the setting and each of the twelve months, climatic features are defined as:
\begin{itemize}
\setlength\itemsep{0em}
\item SDMN: solar radiation, dry days, monthly average, MJ m-2 d-1
\item SDSD: solar radiation, dry days, monthly standard deviation, MJ m-2 d-1
\item SWMN: solar radiation, wet days,monthly average, MJ m-2 d-1
\item SWSD: solar radiation, wet days,monthly standard deviation, MJ m-2 d-1 
\item XDMN: temperature maximum, dry days,monthly average, \textdegree{}C
\item XDSD: temperature maximum, dry days,standard deviation, \textdegree{}C
\item XWMN: temperature maximum, wet days,monthly average, \textdegree{}C
\item XWSD: temperature maximum, wet days,standard deviation, \textdegree{}C
\item NAMN: temperature minimum, all days, monthly average, \textdegree{}C
\item NASD: temperature minimum, all days, monthly standard deviation, \textdegree{}C
\item ALPHA: monthly value of gamma distribution shape parameter
\item RTOT: rainfall total, mm month-1
\item PDW : probability of a dry-wet sequence
\item RNUM: rainy days, \# month-1
\end{itemize}
% \paragraph{Soil features}We consider 7 different soil settings, each soil having the following features:
% \begin{itemize}
% \setlength\itemsep{0em}
% \item DEPTH: soil rooting depth, cm
% \item SLDR: soil permeability, unitless
% \item SLRO: soil runoff curve, unitless
% \item PAW : total soil plant available water, mm
% \item SLOC: soil organic content, massic fraction
% % \item cation exchange capacity, cmol(+)/kg
% \end{itemize}
% \RG{you can see examples in present overleaf's "data\_example" folder}
% \paragraph{Context feature vector.} A field context feature vector is a combination of 1 of the 3 climatic settings and 1 the 7 soil settings.
