# Supplementary material for: Towards an efficient and risk aware strategy for guiding farmers in identifying best crop management
Source: arXiv:2210.04537 source file (2022-10-10)
Supplement: Supplementary file 3 [file old.tex]

\subsection{Essential features}
\textbf{The overarching idea is to reuse CVTS as possible!} \\
\fcolorbox{red}{yellow}{%
\minipage[t]{\dimexpr.9\linewidth-2\fboxsep-2\fboxrule\relax}
\begin{enumerate}
    \item batch recommendation \\
    $\hookrightarrow$ we know that a season lasts for 6 months, and in best settings we can  grow a crop twice a year. We need to run the algo over batches of farmers to be able to collect enough data to be efficient
    \item each field is a context \\
    $\hookrightarrow$ we will collect points from different fields which may greatly impact the results (e.g. shallow poorly fertile soil, deep fertlile soil). We absolutely need to be able to take this context into account. We can see this as: \textbf{observed yield = f(sowing date, field)}
    \item we would like to take advantage as possible of extra information \\
     $\hookrightarrow$ could be a static dataset, or through simulations. The more I manipulate simulators, the less I believe in their ability to model with fidelity. They are more suited to roughly model field dynamics. After all, maybe a static offline data set, with ground observed planting date, context and yield would be the best to initialize the bandit (e.g. of size batch size).
    \item Integrate compliance \\
     $\hookrightarrow$ an experimented farmer, or a farmer that has learnt may be less prone to follow a recommendation and then penalize exploration strategy. Ideally we may a have a meta bandit to deal with compliance.
    \item[(5.)] An extra but interesting feature, would be able to match past similar weather time series to guide the exploration. \\
    $\hookrightarrow$ often, one may use "case based reasoning" i.e. I will act based on the closest situation I met in the past.
\end{enumerate}
\endminipage
}

\paragraph{}We want to provide support for planting date choice to a pool of $M$ farmers. Before making recommendations, we pre-learn  the CDFs of $K$ yield distributions thanks to a crop-simulator, each CDF corresponding to a given planting date. Thus, we have a set $\mathcal{C}_{\text{sim}}$ of $K$ empirical CDFs, estimated from $n_{\text{sim}}$ points. Given this prior knowledge, we want to produce recommendations for real-world conditions, corresponding to a set $\mathcal{C}_{\text{ground}}$ of $K$ true CDFs.

\paragraph{Simplified Hypothesis}We suppose that the batch size $M$ is fixed. We suppose that all farmers exactly follow recommendations. We suppose that the corresponding distributions of $\mathcal{C}_{\text{ground}}$ are stationary. We suppose that $\mathcal{C}_{\text{ground}}$ are the same for all farmers.

\paragraph{Alternate Realistic Hypothesis (sorted by importance)}
\begin{enumerate}
    \item We suppose that farmers follow the recommendations with probability $\pi$, else they randomly pick an action in $K$.
    \item We suppose that there is a variability for $\mathcal{C}_{\text{ground}}$ at farmer level, e.g. farmers' soils are not exactly the same, thus there is an additional noise with reward observations.
    \item We suppose that the batch size $M$ is constant, but that once a learner's averaged rewards is greater than a threshold $y_{\text{min}}$, the learner is replaced by a new one with an empty reward history.
    \item We suppose that $\mathcal{C}_{\text{ground}}$ can change with time.
\end{enumerate}


\paragraph{Constrains}We want to minimize the regret at Community level, with the constraint of "fair exploration", e.g. we cannot recommend twice an high-estimated-gap-action to the same farmer.

\paragraph{Regret measure}We measure the regret by sub-sampling observations in proportion of bandit's stochastic policy. We want to minimize the regret at level community, e.g. for each round, the regret is summed over all individuals, for actions corresponding to the ones recommended.

\section{First technical ideas}

\subsection{Recommendations to a batch of $M$ farmers}

The B-CVTS algorithm seems directly suitable to provide a batch of $M$ recommendations as it is a sequential randomized algorithms. At the beginning of a round $t$, the algorithm will tune all of its parameters according to the history of all the $(t-1)M$ past observations. If we assume that all $M$ farmers have the same action choices and the same $\alpha$ for CVaRs then the algorithm will simply sample $M$ steps of B-CVTS and dispatch the recommendations on the set of farmers. Interestingly, the algorithm can perfectly handle the fact that the parameter $\alpha$ of each farmer is different.

I think that splitting the risk between farmers can first be made independently of the CVTS algorithm. A solution could be to compute a metric to compare the risk taken by each farmer with the information available by the algorithm. If we write $\widetilde \Delta_{t,i}$ the estimated gaps with the information available at the beginning of round $t$ and $A_t^m$ the action suggested to the farmer $m$ at round $t$ we could rank the farmers according to the quantities

\[D_t^m = \sum_{s=1}^{t} \widetilde \Delta_{s,A_{s}^m}^2 \;,\]

then the set of the $M$ actions that will be played at round $t$, $\mathcal{A}_t= (a_{t}^1, \dots, a_t^M)$ is ranked according to the values of the estimated gap, and the actions with higher estimated gaps are distributed to the farmers with the lowest $D_{t-1}^m$.

\subsection{Use and evaluation of $\mathcal{C}_{sim}$}

$\mathcal{C}_{sim}$ provides $K$ cdf $F_1, F_2,\dots, F_K$ that can be used by the B-CVTS algorithm. As they are empirical evaluations they are not exactly the distributions of the simulator, but we assume that $n_{sim}$ is large enough so that they are quite close. A first intuitive way to use them in B-CVTS could be to initialize the algorithm by drawing weights from a uniform Dirichlet, used to re-weight the sums of simulated observations $X_{k, 1}, \dots, X_{k, n_{sim}}$. However, if $n_{sim}$ is large this is burdensome and the simulations would completely out-weight the real observations. What we propose instead is 1) to discretize the observations from the simulator, and obtain a set of values $(x_{k, 1}, \dots, x_{k, n_k})$ and a set of frequencies $(f_{k, 1}, f_{k, n_k})$. There are several possibilities for the discretization step, the two most intuitive are fixed steps or fixed frequencies (bins of size $\delta_x$ between the min and max values in the first case, bins containing a fraction $1/n$, with a fixed $n$). I would tend to prefer the second as it allow to get the same size for each distribution even if their range differ. Let say that for each arm $k$ with have two vectors $X_k^0=(x_{k, 1}, \dots, x_{k, n})$ and $f_k^0 = (1/n, \dots, 1/n)$. We addressed the problem of the complexity by reducing $n_{sim}$ to $n$, but we still have to address the problem of the weight of the prior.

With this new definition, the entire simulator distribution has the weight of $1$ observation in B-CVTS. This is not very informative and we may like to give it more weight. I think one intuitive way to do that is to think about the weight the prior should have in terms of the number of realistic observations it should represent. Namely, we may define a value $N$ and use $N f_k^0$ instead of $f_k^0$ in the B-CVTS algorithm. 
There are in my opinion two challengers. The first is the choice of $N$: is it possible to quantify the trade-off between a high confidence in the prior ($N$ large) and no confidence at all ($N=0$)? We suffer the same problem as in switching bandits: if we set $N$ too large we will only draw the optimal arm defined by the prior and will only be able to notice the gap between the estimation of this arm and its true distribution in reality. Hence, if an arm is under-estimated and is optimal in practice it will take a very long time to be noticed. A possibility could be to define an initial risk budget $\sum_{m=1}^M D_1^m \leq B$, and to perform the first B-CVTS step with an increasing size for $N$ while the initial risk measure is below the risk budget.

Once $N$ is fixed we have the choice to let it fixed or to adapt it sequentially. A fixed $N$ does not seem to be a bad solution is the simulator distributions are quite close to the true distribution, but can be a problem if we find out that the distributions do not match. The problem is to quantify this "distribution mismatch". A first intuitive possibility could be to compute a distance between the empirical distributions and the simulator distributions. However, if $M$ is not very large with reasonable probability the distributions will not match and hence we may disqualify the simulator because of bad luck. A smoother way to estimate this could be to think similarly as with the lower bounds: for instance, we could compute the "closest" model from $f_1, \dots, f_K$ that would make $k$ the optimal arm. Then we could compute the ratio of the likelihood of the observation in the simulated model and in these alternative models. If the ratio is greater than $1$ then the simulated model is more plausible than the model where $k$ is the optimal arm and we will stay confident in the prior. Otherwise, we may reduce the weight of the prior for distribution $k$. The way to reduce this weight has to be defined. 

\paragraph{Example} We assume that we have distributions $F_1, \dots, F_K$ of respective means $\mu_1 > \mu_2 > \dots > \mu_K$. For each $k\geq 2$ we can compute 
\[G_k = \inf_{G\in \cF} \left\{\KL(F_k, G): \bE_{X \sim G}(X) \geq \mu_1 \right\}  \;,\]

and then define 
\[w_k = \min \left(\frac{\bP_{F_k}(x_1, \dots, x_{N_k(t)})}{\bP_{G_k}(x_1, \dots, x_{N_k(t)})}, 1 \right) = \min \left( \prod_{i=1}^{N_k(t)} \frac{\bP_{F_k}(x_i)}{\bP_{G_k}(x_i)}, 1\right) \;, \]
and define re-weight the prior as $N_0 w_k f_k^0$ for each arm $k\geq 2$. For arm $1$ we can do the same, but consider $\bE_{X \sim G}(X)\leq \mu_2$ in the infimum. The interest of this weighting scheme will depend on the smoothness of $w_k$, in particular I don't exactly how the probability can be smooth when the distributions are close.
